# Supplementary material for: The origin of chirality induced spin selectivity in photo-induced electron transfer
Source: arXiv:2106.06554 source file (2021-06-11)
Supplement: Supplementary file 1 [file si.pdf]

# Supporting Information to "The origin of chirality induced spin selectivity in photo-induced electron transfer"

Thomas P. Fay[1,a)] and David T. Limmer[1,2,3,4]

[1)]Department of Chemistry, University of California, Berkeley, CA 94720, USA

[2)]Kavli Energy Nanoscience Institute at Berkeley, Berkeley, CA 94720, USA

[3)]Chemical Sciences Division, Lawrence Berkeley National Laboratory, Berkeley, CA 94720, USA

[4)]Materials Science Division, Lawrence Berkeley National Laboratory, Berkeley, CA 94720, USA

## I. SIMULATION METHODS

The HEOM method is used to perform simulations on a three state model, where the diabatic potential energy surfaces are treated as a set of harmonic oscillators. This model is given by the following Hamiltonian, which can be split into bath kinetic energy $\hat{T}_{\mathrm{b}}$, diabatic potential terms $\hat{V}_{\mathrm{A}}$, with $\mathrm{A} = \mathrm{S}_1, \mathrm{CT}_1$ and $\mathrm{CT}_2$, and the diabatic+spin-orbit coupling term $\hat{V}_{\mathrm{ET}}$,

$$\hat{H} = \hat{T}_{\mathrm{b}} + \hat{V}_{\mathrm{S}_1} + \hat{V}_{\mathrm{CT}_1} + \hat{V}_{\mathrm{CT}_1} + \hat{V}_{\mathrm{ET}} \tag{S.1a}$$

$$\hat{V}_{\mathrm{S}_1} = |\mathrm{S}_1\rangle\langle\mathrm{S}_1|\,\hat{V}_{\mathrm{b}} \tag{S.1b}$$

$$\begin{aligned}\hat{V}_{\mathrm{CT}_1} = {} & |\mathrm{CT}_1,\mathrm{S}\rangle\langle\mathrm{CT}_1,\mathrm{S}|\left(\hat{V}_{\mathrm{b}} + E_{\mathrm{CT}_1} + J + \hat{B}_{\mathrm{CT}_1}\right)\\ & + |\mathrm{CT}_1,\mathrm{T}_0\rangle\langle\mathrm{CT}_1,\mathrm{T}_0|\left(\hat{V}_{\mathrm{b}} + E_{\mathrm{CT}_1} - J + \hat{B}_{\mathrm{CT}_1}\right)\end{aligned} \tag{S.1c}$$

$$\hat{V}_{\mathrm{CT}_2} = \left(|\mathrm{CT}_2,\mathrm{S}\rangle\langle\mathrm{CT}_2,\mathrm{S}| + |\mathrm{CT}_2,\mathrm{T}_0\rangle\langle\mathrm{CT}_2,\mathrm{T}_0|\right)\left(\hat{V}_{\mathrm{b}} + E_{\mathrm{CT}_2} + J + \hat{B}_{\mathrm{CT}_2}\right) \tag{S.1d}$$

$$\begin{aligned}\hat{V}_{\mathrm{ET}} = {} & \Gamma_{\mathrm{DA}_1}\left(\cos\theta\,|\mathrm{CT}_1,\mathrm{S}\rangle\langle\mathrm{S}_1| + i\sin\theta\,|\mathrm{CT}_1,\mathrm{T}_0\rangle\langle\mathrm{S}_1|\right)\\ & + \Gamma_{\mathrm{A}_1\mathrm{A}_2}\left(|\mathrm{CT}_2,\mathrm{S}\rangle\langle\mathrm{CT}_1,\mathrm{S}| + |\mathrm{CT}_2,\mathrm{T}_0\rangle\langle\mathrm{CT}_1,\mathrm{T}_0|\right) + \mathrm{h.c.}\end{aligned} \tag{S.1e}$$

where $\hat{T}_{\mathrm{b}} = \sum_k \hat{p}_k^2/(2m_k)$ is the bath kinetic energy, $\hat{V}_{\mathrm{b}} = \sum_k (m_k\omega_k^2/2)\hat{q}_k^2$ is the unshifted harmonic potentials, $\hat{B}_{\mathrm{CT}_1} = \sum_k c_k\hat{q}_k$ is the bath coupling operator for $\mathrm{CT}_1$, $\hat{B}_{\mathrm{CT}_2} = [(\sqrt{\lambda_{\mathrm{ET1}}} + \sqrt{\lambda_{\mathrm{ET2}}})/\sqrt{\lambda_{\mathrm{ET1}}}]\hat{B}_{\mathrm{CT}_1}$ is the bath coupling operator for $\mathrm{CT}_2$, and the state energies are related to the reorganization energies and free energy changes by $E_{\mathrm{CT}_1} = \Delta G_{\mathrm{ET1}} + \lambda_{\mathrm{ET1}}$, and $E_{\mathrm{CT}_2} = \Delta G_{\mathrm{ET1}} + \Delta G_{\mathrm{ET2}} + (\sqrt{\lambda_{\mathrm{ET1}}} + \sqrt{\lambda_{\mathrm{ET2}}})^2$. The spectral density, $\mathcal{J}(\omega) = (\pi/2)\sum_k (c_k^2/(m_k\omega_k))\delta(\omega - \omega_k)$, which fully defines the harmonic bath, is taken to be of Debye form $\mathcal{J}(\omega) = 2\lambda_{\mathrm{D}}\gamma_{\mathrm{D}}\omega/(\gamma_{\mathrm{D}}^2 + \omega^2)$

---

[a)]Electronic mail: tom.patrick.fay@gmail.com

with $\lambda_{\mathrm{D}} = \lambda_{\mathrm{ET1}}$. The $\mathrm{T}_{\pm}$ states of the CT states are uncoupled from this set of ET states in this model, so we do not need to include them.

HEOM calculations are performed using the frequency based cut-off scheme for the hierarchy of auxiliary density operators (ADOs) described in Ref. 1, along with with ADO rescaling scheme in Ref. 2. A cut-off of $\Gamma = 250\gamma_{\mathrm{D}}$ is used, generating a hierarchy of 375 ADOs with contributions from the first two the Matsubara modes, and the remaining ADOs are treated with the Markovian approximation.[3] The equations of motion are integrated using the short iterative Arnoldi method[4] with a Krylov subspace dimension of 16 and an adaptive time step, in which the Krylov subspace is updated when the coefficient of the last Krylov vector is greater than $\epsilon = 10^{-11}$ times the norm of the HEOM state vector.

The second order master equation rate constants are given by

$$k_{\mathrm{A}\to\mathrm{B}} = \frac{2\Gamma_{\mathrm{AB}}^2}{\hbar^2} \mathrm{Re}\int_0^\infty \mathrm{d}t\, \frac{\mathrm{Tr}_{\mathrm{b}}[e^{-\beta \hat{H}_{\mathrm{A}}^{\mathrm{b}}} e^{+i\hat{H}_{\mathrm{A}}^{\mathrm{b}} t} e^{-i\hat{H}_{\mathrm{B}}^{\mathrm{b}} t}]}{\mathrm{Tr}_{\mathrm{b}}[e^{-\beta \hat{H}_{\mathrm{A}}^{\mathrm{b}}}]}, \tag{S.2}$$

where $\hat{H}_{\mathrm{A}}^{\mathrm{b}}$ is the nuclear bath Hamiltonian for state A, $\hat{H}_{\mathrm{A}}^{\mathrm{b}} = \hat{T}_{\mathrm{b}} + \hat{V}_{\mathrm{b}} + E_{\mathrm{A}} + \hat{B}_{\mathrm{A}}$, and $\Gamma_{\mathrm{AB}}$ is the coupling between states A and B. Similarly the shift term is given by,

$$\delta\epsilon = \frac{\Gamma_{\mathrm{DA}_1}^2}{\hbar} \mathrm{Im}\int_0^\infty \mathrm{d}t\, \frac{\mathrm{Tr}_{\mathrm{b}}[e^{-\beta \hat{H}_{\mathrm{CT1}}^{\mathrm{b}}} e^{+i\hat{H}_{\mathrm{CT1}}^{\mathrm{b}} t} e^{-i\hat{H}_{\mathrm{CT2}}^{\mathrm{b}} t}]}{\mathrm{Tr}_{\mathrm{b}}[e^{-\beta \hat{H}_{\mathrm{CT1}}^{\mathrm{b}}}]}. \tag{S.3}$$

For the harmonic bath model these depend only on the spectral density $\mathcal{J}(\omega)$, second order master equation parameters are calculated using the expressions in Ref. 5, with the spectral density discretized into 2000 modes using the standard procedure.[6] The full expression for the integrand in the above expressions is,

$$\begin{aligned}&\frac{\mathrm{Tr}_{\mathrm{b}}[e^{-\beta \hat{H}_{\mathrm{A}}^{\mathrm{b}}} e^{+i\hat{H}_{\mathrm{A}}^{\mathrm{b}} t} e^{-i\hat{H}_{\mathrm{B}}^{\mathrm{b}} t}]}{\mathrm{Tr}_{\mathrm{b}}[e^{-\beta \hat{H}_{\mathrm{A}}^{\mathrm{b}}}]} \\ &\qquad = \exp\left(i\frac{\Delta E_{\mathrm{AB}} t}{\hbar} + \frac{1}{\pi\hbar}\int_0^\infty \frac{\mathcal{J}_{\mathrm{AB}}(\omega)}{\omega^2}\left[\coth\left(\frac{\hbar\omega}{2k_{\mathrm{B}}T}\right)(1-\cos(\omega t)) - i\sin(\omega t)\right]\mathrm{d}\omega\right),\end{aligned} \tag{S.4}$$

where $\Delta E_{\mathrm{AB}} = -\Delta G_{\mathrm{A}\to\mathrm{B}}$, and $\mathcal{J}_{\mathrm{AB}}(\omega)$ is the spectral density with the reorganization energy, set to that for the $\mathrm{A} \to \mathrm{B}$ electron transfer. The master equations themselves form a linear system of equations are numerically integrated by directly exponentiating the generator for this system of equations.

## II. DEPHASING AND RECOMBINATION PROCESSES

Let us briefly consider two processes which could affect the spin polarization observed in this mechanism: competing electron recombination reactions such as $CT_1 \xrightarrow{k_{ET0}} S_0$, and singlet-triplet dephasing in intermediate CT states. Competing back reactions will both lead to singlet-triplet decoherence in the intermediate $CT_1$ state at a rate of $k_{ET0}/2$, but they will also reduce the yield of the final $CT_2$ state but removing, so the spin polarization, relative to the final yield can increase or decrease. Singlet-triplet dephasing will lead to additional decay of singlet-triplet coherences at a rate $k_{STD}$, which will reduce the final spin polarization. In the limit where $|2J| \gg |\delta\epsilon|$, by solving a modified version of Eq. (4) the spin polarization relative to the $CT_2$ yield is found to be,

$$\frac{\langle \Delta P_z \rangle}{\phi_{CT_2}} = -\frac{\sin(2\theta) k_{ET2} \left(\frac{2J}{\hbar}\right)\left(1 + \frac{k_{ET0}}{k_{ET2}}\right)}{\left(\frac{\sin^2\theta k_{ET0}}{k_{ET2}} + 1\right)\left(\left(\frac{2J}{\hbar}\right)^2 + \left(\frac{k_{ET0}}{2} + k_{ET2} + k_{STD}\right)^2\right)} \quad (S.5)$$

so we see that the back electron transfer rate $k_{ET0}$ can either increase or decrease the spin polarization, but the singlet triplet-dephasing rate will always decrease the spin polarization.

## III. CONNECTION TO CIDEP

The mechanism of CISS described here is closely related to the mechanism by which Chemically Induced Dynamic Electron Polarization (CIDEP) can be generated in singlet born radical pairs at large applied magnetic fields.[7] CIDEP can be generated by the combination of the $\Delta g$ mechanism, in which a radical pair is generated in a coherent but non-polarized superposition of $|S\rangle$ and $|T_0\rangle$ states by different precession frequencies of the radical electron spins in a large applied magnetic field. The resulting state can then become transiently spin polarized if the radical pair has a strong exchange coupling, and this can be frozen out if the radical pair diffuses apart into a configuration with a very weak exchange coupling.[7,8] In this mechanism the $\Delta g$ mechanism plays a similar role at large very high applied magnetic fields to the spin-orbit coupling mediated electron transfer, effectively rotating one electron spin relative to the other.

[1] Dijkstra, A. G.; Prokhorenko, V. I. Simulation of photo-excited adenine in water with a hierarchy of equations of motion approach. *J. Chem. Phys.* **2017**, *147*, 064102.

[2] Shi, Q.; Chen, L.; Nan, G.; Xu, R.-X.; Yan, Y. Efficient hierarchical Liouville space propagator to quantum dissipative dynamics. *J. Chem. Phys.* **2009**, *130*, 084105.

[3] Ishizaki, A.; Tanimura, Y. Quantum Dynamics of System Strongly Coupled to Low-Temperature Colored Noise Bath: Reduced Hierarchy Equations Approach. *J. Phys. Soc. Japan* **2005**, *74*, 3131–3134.

[4] Pollard, W. T.; Friesner, R. A. Solution of the Redfield equation for the dissipative quantum dynamics of multilevel systems. *J. Chem. Phys.* **1994**, *100*, 5054–5065.

[5] Fay, T. P.; Lindoy, L. P.; Manolopoulos, D. E. Spin-selective electron transfer reactions of radical pairs: Beyond the Haberkorn master equation. *J. Chem. Phys.* **2018**, *149*, 064107.

[6] Wang, H.; Thoss, M. Theoretical study of ultrafast photoinduced electron transfer processes in mixed-valence systems. *J. Phys. Chem. A* **2003**, *107*, 2126–2136.

[7] Hore, P. J.; Joslin, C. G.; McLauchlan, K. A. The role of chemically-induced dynamic electron polarization (CIDEP) in chemistry. *Chem. Soc. Rev.* **1979**, *8*, 29.

[8] Hore, P. Transfer of spin correlation between radical pairs in the initial steps of photosynthetic energy conversion. *Mol. Phys.* **1996**, *89*, 1195–1202.
